# Supplementary material for: Near-unity radiative quantum efficiency of excitons in carbon nanotubes
Source: arXiv:2102.10718 ancillary file (2021-02-22)
Supplement: Supplementary file 1 [file radiativeqe-supplementary.pdf]

Supplementary Information

# Near-unity radiative quantum efficiency of excitons in carbon nanotubes

H. Machiya[1,2], D. Yamashita[3], A. Ishii[1,3], and Y. K. Kato[1,3]

[1] *Nanoscale Quantum Photonics Laboratory, RIKEN Cluster for Pioneering Research, Saitama, 351-0198, Japan*

[2] *Department of Electrical Engineering, The University of Tokyo, Tokyo, 113-8656, Japan*

[3] *Quantum Optoelectronics Research Team, RIKEN Center for Advanced Photonics, Saitama, 351-0198, Japan*

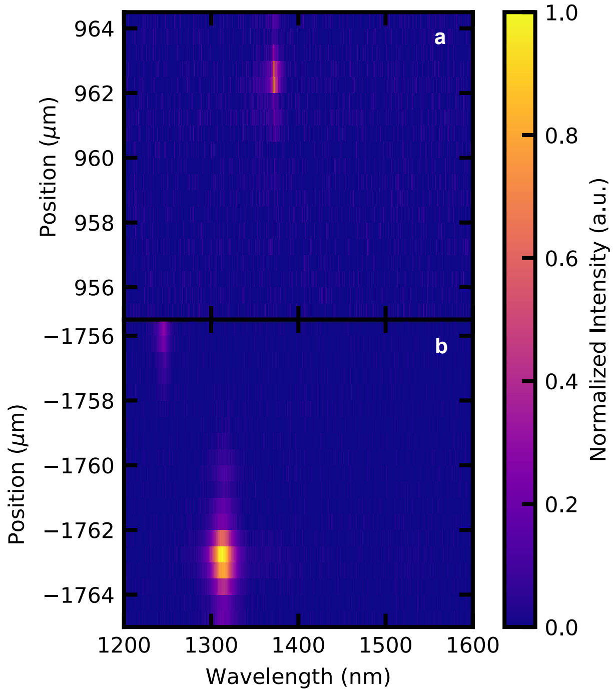


**Supplementary Figure 1** PL line scans along nanobeam cavities for (a) a coupled and (b) an uncoupled device. Excitation power and wavelength are 200 µW and 800 nm, respectively. Laser polarization is perpendicular to the nanobeam axis.

**Supplementary Table 1** Summary of the Purcell and acceleration factors for 15 devices shown in Fig. 5.

| | Chirality | $I_{cav}$ (a.u.) | $I_{CNT}$ (a.u.) | $\tau_1$(ps) | $\tau_2$(ps) | $L$ (μm) | $F$ | $A$ | $\eta$ |
|---|---|---|---|---|---|---|---|---|---|
| 1 | (9,8) | 3680 ± 950 | 47660 ± 2170 | 34.8 ± 0.3 | 586 ± 5 | 2.49 ± 0.13 | 0.84 ± 0.22 | 1.82 ± 0.09 | 0.98 ± 0.11 |
| 2 | (9,8) | 8140 ± 350 | 8540 ± 580 | 20.7 ± 0.1 | 307 ± 4 | 1.82 ± 0.13 | 5.81 ± 1.13 | 2.64 ± 0.16 | 0.28 ± 0.11 |
| 3 | (11,6) | 22870 ± 1440 | 68540 ± 3680 | 26.7 ± 3.3 | 330 ± 3 | 1.85 ± 0.04 | 3.63 ± 0.35 | 2.24 ± 0.28 | 0.34 ± 0.16 |
| 4 | (9,7) | 39920 ± 3690 | 53950 ± 6950 | 15.4 ± 0.03 | 384 ± 16 | 1.87 ± 0.08 | 8.98 ± 1.93 | 4.21 ± 0.12 | 0.36 ± 0.06 |
| 5 | (9,8) | 7050 ± 350 | 21660 ± 1100 | 24.7 ± 3.8 | 554 ± 10 | 2.42 ± 0.13 | 4.14 ± 0.28 | 2.54 ± 0.42 | 0.37 ± 0.23 |
| 6 | (11,6) | 16810 ± 2080 | 42050 ± 3320 | 31.8 ± 1.5 | 272 ± 3 | 1.43 ± 0.04 | 4.50 ± 0.89 | 3.00 ± 0.09 | 0.44 ± 0.04 |
| 7 | (11,6) | 8200 ± 650 | 13630 ± 1010 | 13.9 ± 0.08 | 257 ± 3 | 1.64 ± 0.04 | 6.56 ± 0.96 | 3.93 ± 0.10 | 0.45 ± 0.04 |
| 8 | (11,6) | 6460 ± 1090 | 22740 ± 2570 | 21.9 ± 0.07 | 301 ± 2 | 1.77 ± 0.04 | 3.16 ± 0.83 | 2.65 ± 0.06 | 0.52 ± 0.03 |
| 9 | (11,6) | 15930 ± 3010 | 66030 ± 6630 | 20.0 ± 2.4 | 299 ± 3 | 1.76 ± 0.04 | 3.60 ± 0.99 | 2.90 ± 0.39 | 0.53 ± 0.16 |
| 10 | (10,8) | 7690 ± 890 | 48650 ± 1970 | 28.4 ± 0.1 | 234 ± 4 | 1.75 ± 0.13 | 1.74 ± 0.25 | 1.94 ± 0.12 | 0.54 ± 0.07 |
| 11 | (9,7) | 6070 ± 370 | 23570 ± 1000 | 17.7 ± 5.0 | 503 ± 5 | 2.13 ± 0.07 | 4.04 ± 0.36 | 3.93 ± 1.12 | 0.73 ± 0.35 |
| 12 | (10,8) | 8580 ± 1330 | 38510 ± 3300 | 20.0 ± 0.2 | 314 ± 5 | 2.01 ± 0.13 | 2.45 ± 0.54 | 3.00 ± 0.17 | 0.82 ± 0.07 |
| 13 | (11,6) | 1390 ± 190 | 13850 ± 710 | 24.7 ± 7.9 | 356 ± 8 | 1.91 ± 0.05 | 1.67 ± 0.27 | 2.49 ± 0.80 | 0.89 ± 0.49 |
| 14 | (9,7) | 5220 ± 550 | 37480 ± 1280 | 23.3 ± 0.5 | 505 ± 8 | 2.13 ± 0.07 | 2.14 ± 0.23 | 2.98 ± 0.10 | 0.93 ± 0.05 |
| 15 | (10,8) | 9340 ± 1140 | 35240 ± 1600 | 15.5 ± 0.07 | 373 ± 4 | 2.18 ± 0.13 | 2.92 ± 0.48 | 4.02 ± 0.22 | 1.03 ± 0.08 |
